# Supplementary material for: Pseudogap to metal transition in the anisotropic two-dimensional Hubbard model
Source: arXiv:1707.09446 ancillary file (2017-07-29)
Supplement: Supplementary file 1 [file PG_supplement.pdf]

# SUPPLEMENTAL MATERIAL
# for
# Pseudogap to metal transition in the anisotropic two-dimensional Hubbard model

J. P. L. Faye
*The Abdus Salam International Center for Theoretical Physics, Strada Costiera 11, 34014 Trieste, Italy*

D. Sénéchal
*Département de physique and Institut Quantique, Université de Sherbrooke, Sherbrooke, Québec, Canada J1K 2R1*
(Dated: July 28, 2017)

In this supplement we provide more data supporting our conclusions and comment further on some of the results shown in the main paper.

### Bath parameters

The pseudogap to metal transition can be best tracked by following the bath parameters $\epsilon_{1,2}$ and $\theta_{1,2}$ as a function of chemical potential. A set of solutions for $U = 7$ and $t_y = 0.8$ is illustrated on Fig. 1. The transition between the pseudogap and metallic phases takes the form of a discontinuity accompanied by a hysteresis loop. The same quantities plotted against the doping $\delta = n-1$ would show a gap, i.e., a forbidden region of doping in which the two phases coexist (contrary to $U = 6$, where the two phases overlap in density).

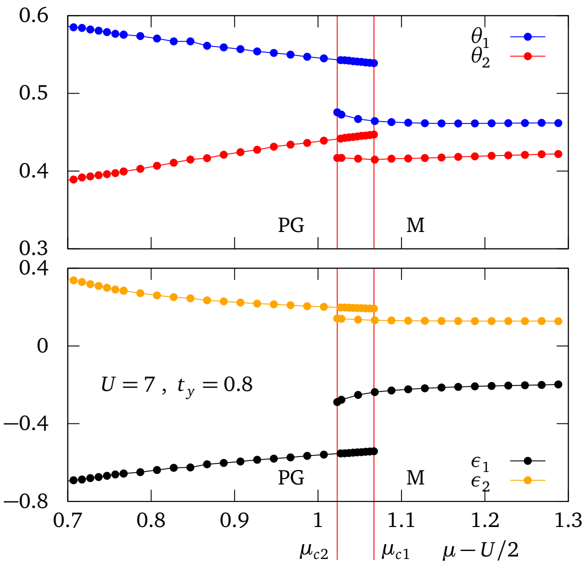


FIG. 1. The four bath parameters $\epsilon_{1,2}$ and $\theta_{1,2}$ as a function of chemical potential for $U = 7$ and $t_y = 0.8$. The scope of the hysteresis loop are indicated by red vertical lines and occur at doping $\delta \sim 9-10\%$.

Figure 2a shows one of the bath parameters ($\epsilon_1$) as a function of chemical potential, this time for several values of $t_y$, ranging from $t_y = 0.5$ to $t_y = 1$. The pseudogap transition is at its most visible in the range $t_y = 0.7$–$0.9$, at least when considering $\epsilon_1$; it has completely disappeared at $t_y = 0.5$. Figure 2c shows the corresponding plot for $U = 6$ and Figure 2c for the bath parameter $\epsilon_2$. The discontinuity in the $t_y = 1$ curve is clearly visible there, even though it is very weak for $\epsilon_1$. Finally, Fig. 2d shows $\epsilon_1$ as a function of chemical potential, for several values of $U$. The hysteresis is most pronounced for values of $U$ close to $U_{c2}$, and practically disappears when $U = 9$. To summarize, the hysteresis loop is widest when $U$ approaches $U_{c2}$ and when $t_y$ approaches 1 (isotropic limit).

### Relation between chemical potential and density

Fig. 2 of the paper shows the relationship between chemical potential and density for several values of $t_y$ at $U = 8$. Fig 4 of this supplement shows the corresponding data for $t_y = 0.8$ for several values of $U$. Once again we see that the hysteresis is more pronounced at lower values of $U$ (close to $U_{c2}$) and is practically gone at $U = 9$.

### Spectral function

Figure 3 shows the spectral function for $U = 6$ and 7% hole doping, where the metallic and pseudogap solutions both exist. The boundaries of the reduced Brillouin zone, associated with the superlattice of plaquettes, is indicated by white dotted lines. In the metallic case, what was the noninteracting Fermi surface rearranges into hole (centered around $k_y = \pm\pi$) and electron (centered around $k_y = 0$) pockets, each pocket having an "intense" and a "ghost-like" vertical arc. Ref. [1, 2] have shown similar plots in the half-filled case. In the pseudogap state, the electron pocket is much attenuated and reduced to a small halo around $\mathbf{k} = (\pm\pi/2, 0)$. However, one needs to be careful not to overinterpret what could be an artifact of the $2 \times 2$ cluster used. The whole approach partially breaks translation symmetry because of the different treatment of the intra-cluster links (within the impurity model) and inter-cluster links (accounted for in $G_0(\mathbf{k}, \omega)$). Thus, wave vectors of the reciprocal superlattice, such as $(\pm\pi, 0)$ and $(0, \pm\pi)$ in the present case, tend to act like effective scattering wave

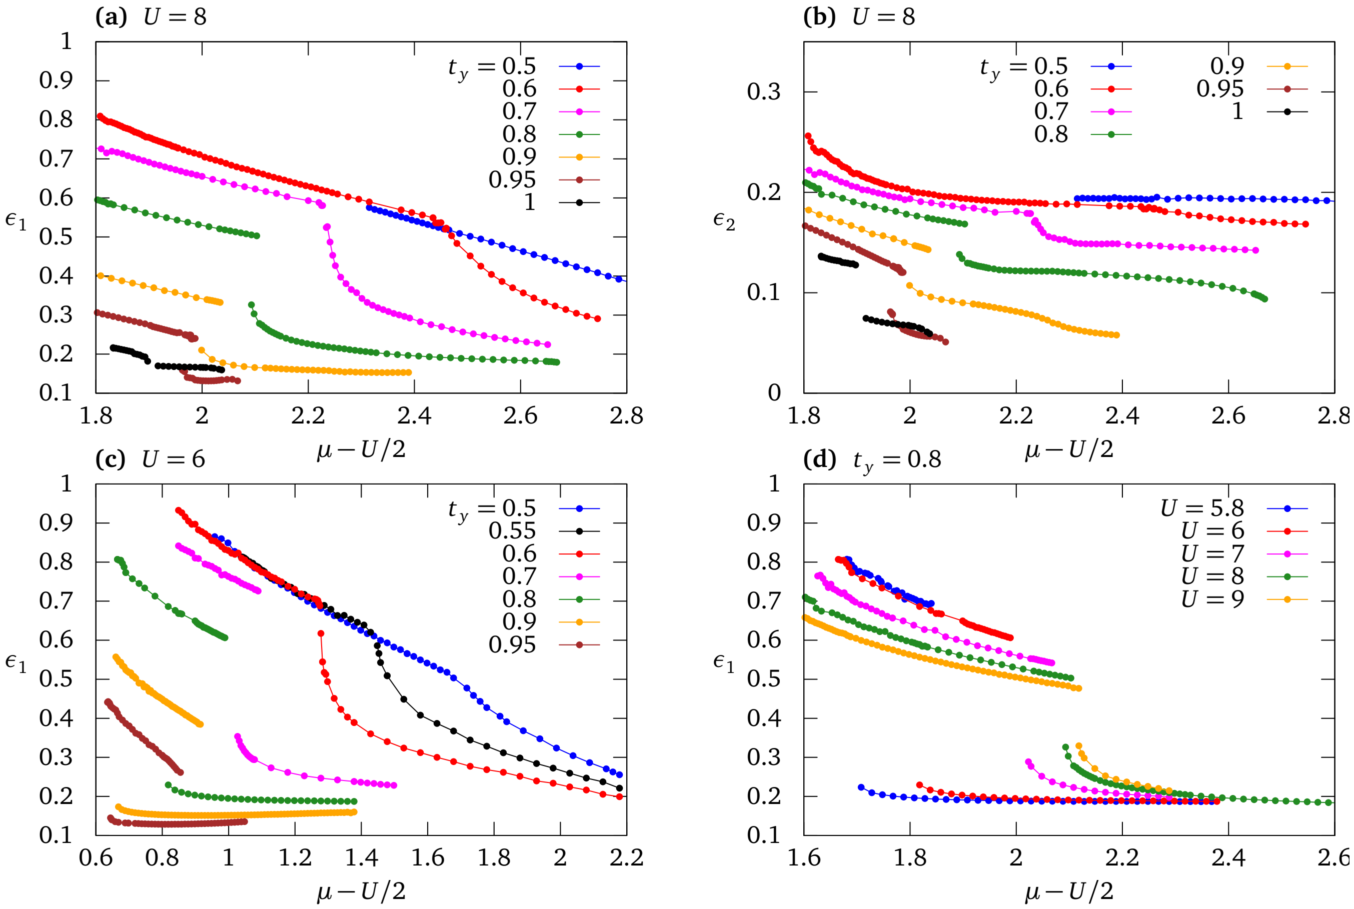


FIG. 2. (a) Bath energy $\epsilon_1$ as a function of $\mu$ for various values of $t_y$ ranging from 0.5 to 1 and $U = 8$. The first-order transition is clearly visible, except at $t_y = 0.5$. It is somewhat weaker close to the isotropic point ($t_y = 1$). (b) Same thing for bath energy $\epsilon_2$. (c) Same thing again, this time for $\epsilon_1$ and $U = 6$. (d) Bath energy $\epsilon_1$ for $t_y = 0.8$ and several values of $U$.

vectors that deplete the spectral weight at points on the Fermi surface separated by them. They can also create artificial ghost structures, like the ones seen here. Thus, it is difficult to distinguish true hot spots, created by the scattering off short-range antiferromagnetic fluctuations at $\mathbf{Q} = (\pm\pi, \pm\pi)$, from artificial ones created by scattering off the reciprocal superlattice, unless we change the cluster size or shape.

This being said, the signature of the pseudogap seen here – the quasi-disappearance of the electron pockets – is not an effect of the cluster shape, since (i) the intense segments of the electron pockets are not related by reciprocal superlattice wave vectors and (ii) it does not occur in the metallic state, which is obtained with the same cluster.

## Phase diagram

Let us comment a little more on the phase scenario illustrated in Fig. 5 of the paper, which we reproduce here on Fig. 5, with three chemical potential scans (noted 1,2,3). Let us first clarify the meaning of the instability curves by describing what happens as one proceeds along the different $\mu$ scans, in both directions. If $\mu$ is decreased along scan (1), one always stays in the metallic phase, which is the most stable solution all along. If, on the other hand, we follow the same scan in the opposite direction, starting from the metastable Mott state at half-filling, then one stays in the Mott state until the green curve is met, at which point one continuously leaves half-filling into the pseudogap state, still in a metastable state, until the dashed blue curve is crossed, at which point one jumps to the metallic state. More precisely, the jump is to a mixture of the pseudogap and metallic states (because the corresponding densities at that value of $\mu$ are not the same) and $\mu$ cannot change until the doping has reached the (larger) value of the metallic state. If $\mu$ is decreased along scan (2), one stays in the metallic state until the red dashed curve, at which point one jumps into a mixture of the Mott insulating state at half-filling with the metallic state, until half-filling is reached (at a constant value of $\mu$), where the pure Mott phase is reached. In the other direction, starting from the Mott state, one crosses continuously into the doped state at

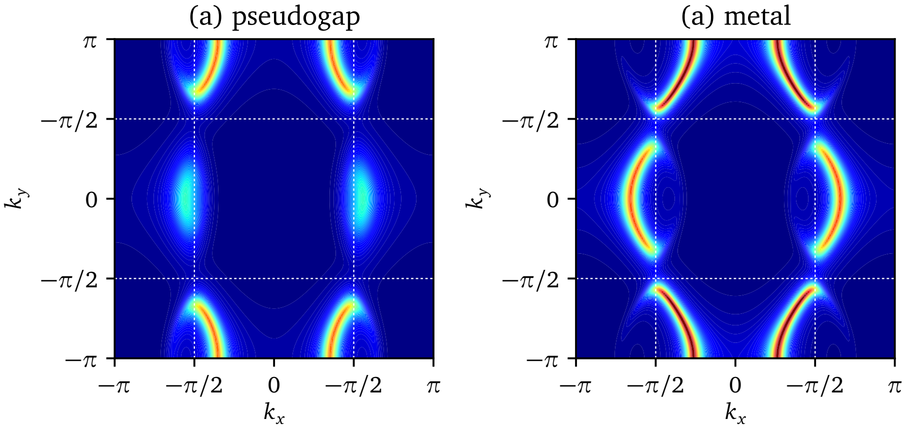


FIG. 3. Spectral function $A(\mathbf{k},0)$ (Fermi level) for $U=6$ and 7% doping. Panel (a) : pseudogap solution. Panel (b) : metallic solution. The pseudogap mainly affects the low $k_y$ region. The scale is the same on both graphs.

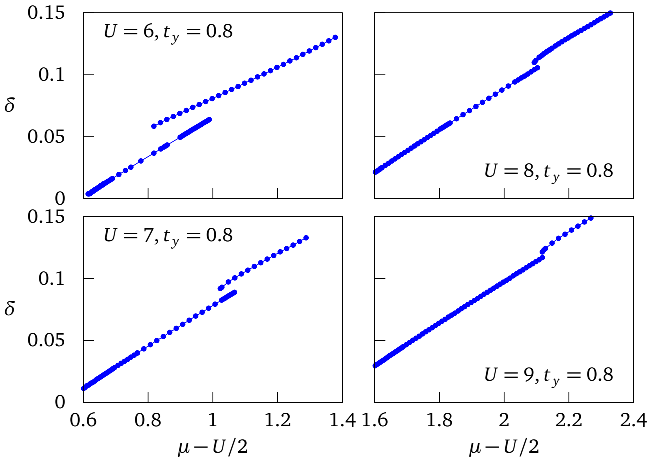


FIG. 4. Relation between chemical potential and doping for $U=6,7,8,9$, $t_y=0.8$. Note that the densities of the two phases overlap at $U=6$, but not at the larger values, which is reflected by the crossing of the instability curves on Fig. 4 of the paper.

the green line, and later the system jumps into the metallic state at the dashed blue curve, as for scan (1). Here too, the jump is into a mixed state with a finite width in density (the blue shaded area of Panel (b)), at fixed chemical potential, until the red boundary of the blue shaded area is reached, at which point one recovers a pure metallic phase. Finally, if $\mu$ is decreased along scan (3), the system goes from the metallic state to a mixture of the metallic state with the pseudogap state at the red dashed curve, and this corresponds to the red shaded area crossed by scan (3) on Panel (b). Before reaching this point in $\mu$, the metallic state went from stable to metastable across the black curve, but this is not an observable transition. Once in the pure pseudogap state, the system reaches half-filling continuously at the green curve. In the other direction, the initial insulating state turns continuously into the pseudogap state across the green curve, until the blue curve is reached, when the system falls into a mixture of the pseudogap and metallic state at a constant $\mu$ (blue shaded area on Panel (b), overlapping with the red shaded area), until the density reaches the pure metallic state value.

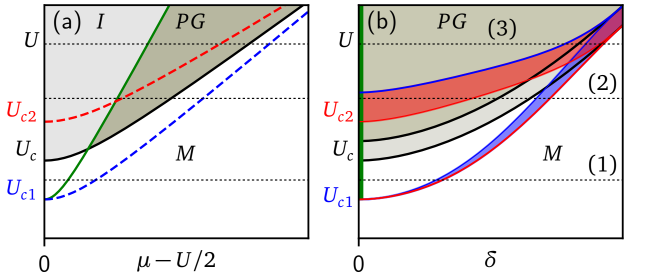


FIG. 5. Phase scenario of Fig. 5 of the paper, with doping or chemical potential scans (1-3) added. See text for explanations.

### Numerical issues

The CDIA proceeds by finding the saddle points of the Potthoff functional Ω (Eq. (3) of the paper). When using bath parameters as variational parameters, Ω is typically a very shallow function of its arguments, and rather difficult to optimize, especially in the PG phase. There is a hierarchy of numerical accuracies that must be followed: the accuracy of the ground state of the impurity problem, found via the Lanczos algorithm, must be the highest, followed by the accuracy of the Green function, also found via a variant of the Lanczos method, followed by the accuracy of Ω itself (typically $10^{-8}$), which is the result of a three-

dimensional integral (we used the CUBA library [3]). At last, the accuracy of the saddle-point search method (the Newton-Raphson method or a quasi-Newton method) must be lower. Typically, we ask for an accuracy of $10^{-3}$ on the bath parameters, with the condition that the gradient of $\Omega$ be smaller than $10^{-4}$.

The isotropic limit $t_y = 1$ is especially difficult numerically. We suspect that this is related to the landscape of $\Omega(\theta, \epsilon)$ at that value. We could obtain a few values at $U = 8$, but left other values of $U$ for future work.

[1] Benjamin Lenz, Salvatore R Manmana, Thomas Pruschke, Fakher F Assaad, and Marcin Raczkowski, "Mott Quantum Criticality in the Anisotropic 2D Hubbard Model," Phys. Rev. Lett., **116**, 086403 (2016), ISSN 10797114.

[2] Marcin Raczkowski and Fakher F Assaad, "Dimensional-crossover-driven Mott transition in the frustrated Hubbard model," Phys. Rev. Lett., **109**, 126404 (2012), ISSN 00319007.

[3] http://www.feynarts.de/cuba/.
